# Supplementary material for: Onset of collective motion in locusts is captured by a minimal model
Source: arXiv:1406.5585 source file (2015-11-06)
Supplement: Supplementary file 1 [file supplementary_material.pdf]

# A MINIMAL MODEL CAPTURES THE ONSET OF COLLECTIVE MOTION IN LOCUSTS

Louise Dyson, Christian A. Yates, Jerome Buhl and Alan J. McKane

## THE EQUATION-FREE METHOD FOR ESTIMATING FOKKER-PLANCK COEFFICIENTS

Although we may expect that a process can be modelled by an SDE, the drift and diffusion terms are often unknown, so that an accurate quantitative model of the behaviour cannot be specified. For example, in the locust data we expect that the behaviour of the alignment, $z(t)$, can be modelled by a discretised SDE [1] of the form:

$$z(t+dt) - z(t) = F(z(t))dt + \sqrt{2D(z(t))}\mathrm{d}W(t), \qquad 0 \le t \le T, \tag{S.1}$$

where $W(t)$ is a standard Wiener process (*i.e.* $\mathrm{d}W(t) = W(t+dt) - W(t) \sim \sqrt{dt}N(0,1)$). This expectation comes from the qualitative similarity between the switching behaviour seen in the time-courses of experimental alignment data and SDEs such as equation (13) of the main text.

In order to estimate the coefficients of the SDE assumed to underlie the data, we appeal to an adaptation of the equation-free technique [2, 3]: the 'Fokker-Planck coefficient estimation approach' [4]. In order to approximate the drift term, $F(z)$, note that the mean of the second term on the right of equation (S.1), $\sqrt{2D(z(t))}\mathrm{d}W$, (averaged over many realisations of this quantity for the same value of $z$) is zero since $\mathrm{d}W \sim \sqrt{dt}N(0,1)$. For a particular value of $z$, this, in combination with equation (S.1), implies that $F(z)$ can be found as

$$F(z) = \lim_{\delta t \to 0} \left\langle \frac{z(t+\delta t) - z(t)}{\delta t} \right\rangle, \tag{S.2}$$

where $\langle\rangle$ represents the average over many instances of the data, beginning with a particular value of $z$, where $\delta t$ is a small-time increment.

Similarly, in order to estimate the unknown diffusion term $D(z)$ we can consider a rearrangement of equation (S.1) as follows:

$$[z(t+\delta t) - z(t)]^2 = F^2\delta t^2 + 2F\sqrt{2D}dW\delta t + 2D\mathrm{d}W^2. \tag{S.3}$$

Upon averaging this quantity over many replicates for the same value of $z$, dividing through by $2\delta t$ and taking the limit as $\delta t \to 0$ we find that

$$D(z) = \frac{1}{2}\lim_{\delta t \to 0} \left\langle \frac{[z(t+\delta t) - z(t)]^2}{\delta t} \right\rangle. \tag{S.4}$$

The equation-free technique was originally designed to allow coarse-graining from microscale models to macroscale models. As such, when attempting to calculate the quantities $F(z)$ and $D(z)$, the domain of values of $z$ for which we wish to calculate the coefficients is first discretised into a set of grid points. For a particular value of $z$, corresponding to a particular grid point in the discretised domain, the microscale model is simply initialised with the correct value of $z$ and run for a short period of time in order to calculate $z(t+\delta t)$. This process can be repeated arbitrarily many times, until good estimates for $F(z)$ and $D(z)$ are found for that particular value of $z$. This process of moving from the microscale model to the macroscale model is known as 'lifting' in the equation-free terminology. When lifting, care must be taken to ensure that the higher moments of the alignment distribution do not adversely affect the approximation [2].

When considering the experimental data, it is not possible to simply initialise the locusts with a particular alignment value, $z(t)$, and run the experiment for a short period of time to calculate $z(t+\delta t)$. Instead we must use the time-course data that we have and wait for the locusts' alignment to fall into a particular grid site of the $z$ domain. We can then find the alignment value a short period of time, $\delta t$, later and calculate a realisation of $z(t+\delta t) - z(t)$, which can be utilised for calculating $F(z)$ and $D(z)$ according to equations (S.2) and (S.4), respectively. Consequently, we cannot guarantee that we will have sufficiently many (or indeed any) realisations over which to average the coefficient approximations for a particular value of $z$. In experiments in which the locusts exhibit coherent switching behaviour we will find that the approximation to the drift and diffusion coefficients are poor at the extreme-high and -low alignment values, which are rarely found in the experimental data, since it is very rare to find absolutely all locusts moving in the same direction.

In order to further justify the use of the Fokker-Planck coefficient estimation approach to approximate the drift and diffusion coefficients of an SDE underlying the experimental data, we test the technique on the known SDE of the model. Recall the SDE (13) of the main text for alignment, $z$:

$$\dot{z} = -2r_1 z + \frac{r_3}{2} z(1-z^2) + \frac{2}{\sqrt{N}} \sqrt{\left(r_1 + \frac{2r_2 + r_3}{4}(1-z^2)\right)}\eta(t). \tag{S.5}$$

Figure S1 ((a) and (b)) demonstrates the results of the application of the coefficient estimation technique in order to estimate the drift and diffusion coefficients of the SDE on a discrete grid of 20 points from $z = -1, \ldots, 1$. The agreement with the known values of the drift (a) and diffusion (b) coefficients is excellent.

We also tested the efficacy of the coefficient estimation technique on the individual-based model (equations (1)-(3) in the main text) in order to determine whether we could derive the coefficients of an assumed underlying SDE. The results are presented in Fig. S1 ((c) and (d)). Again the approximation to both coefficients is good. The approximation is poorest at the extreme values of alignment and in the low values of alignment where the simulation spends least time (see the stationary probability distribution in Fig. 3 of the main text) and hence we have fewer realisations of the quantities given in equations (S.2) and (S.4) over which to average.

For both the individual-based model and the SDE it would have been possible to find more accurate values of the drift and diffusion coefficients at the discrete alignment values which are visited less often by initialising our simulation with those particular values of alignment and running the simulation for the required short period of time as in the traditional equation-free technique. However, since we are not at liberty to do this for the experimental data, it makes sense to use the same technique we will use in that situation on the simulation data in order to show that it is just as effective.

## DRIFT AND DIFFUSION COEFFICIENTS DERIVED FROM THE DATA

Figure S2 displays the equation-free estimation of the drift and diffusion coefficients, described above, applied to experimental data for a range of locust numbers from 5 ((a) and (b)) to 40 ((s) and (t)). When calculating the coefficients we assume that the diffusion coefficient is an even function about $z = 0$ and that the drift coefficient is an odd function about $z = 0$, so that we may average the values obtained over positive and negative alignments to obtain symmetric drift and diffusion coefficients. The assumption is justified by arguing that the derived FPE (equation (9) of the main text) for $P(z,t)$ should be the same as that for $P(-z,t)$, due to the symmetry of the system. Consequently we must have $F(z) = -F(-z)$ and $D(z) = D(-z)$. For low population numbers ($N < 10$) we divide the alignment variable, $z$, into $N+1$ grid points. However, at high population numbers ($N \geq 10$) this would result in a very noisy estimate for the coefficients, since more grid points mean that the system spends less time at each point. We therefore take 11 grid points for $N \geq 10$.

The drift coefficient is generally cubic in shape and the diffusion coefficient takes the shape of a concave polynomial of even order. As described in the main text, this shape is consistent with that given by the IBM (equations (1)-(3) of the main text). The drift coefficient has a pair of non-zero turning points (corresponding to steady states in the purely deterministic system), and these are modified by the noise term with a strength given by the diffusion coefficient. There is more noise in the middle of the domain, where the diffusion coefficient is maximal. This pushes the system away from areas in which there is a large amount of noise, so that the steady states given by the analogous deterministic equation may not be the area in which the system is most likely to reside.

## EXPERIMENTALLY DERIVED STATIONARY PROBABILITY DISTRIBUTIONS

In Fig. S3, for each value of $N$, an approximate SPD is obtained by appropriately binning the data to form a histogram. This is compared with our analytical prediction using the fitted reaction rates given in Table I.

[1] This discretisation is of the Euler-Maruyama type.

[2] I. G. Kevrekidis, C. W. Gear, J. M. Hyman, P. G. Kevrekidis, O. Runborg, and C. Theodoropoulos, Comm. Math. Sci. **1**, 715 (2003).
[3] R. Erban, I. G. Kevrekidis, D. Adalsteinsson, and T. C. Elston, J. Chem. Phys. **124**, 084106:1 (2006).

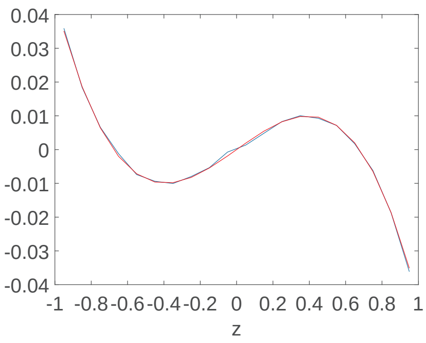


(a)Drift coefficient from SDE

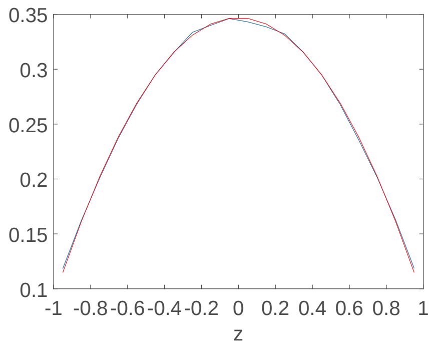


(b)Diffusion coefficient from SDE

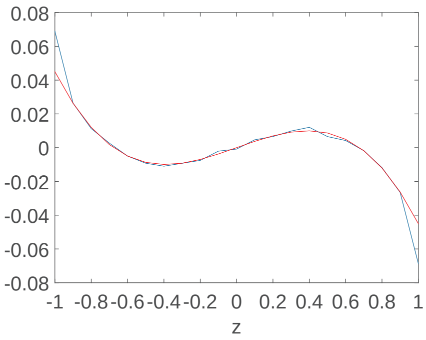


(c)Drift coefficient from IBM

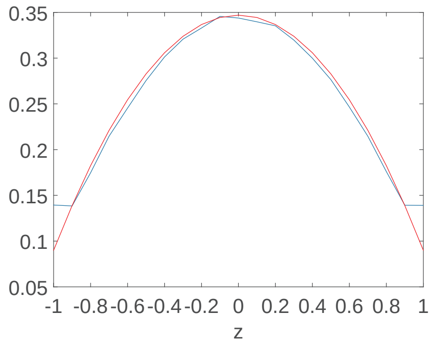


(d)Diffusion coefficient from IBM

FIG. S1. Applying the coefficient estimation technique to simulated data generated from ((a) and (b)) a known SDE (equation (S.5)) and ((c) and (d)) the underlying IBM (equations (1)-(3) of the main text). The estimated drift ((a) and (c)) and diffusion ((b) and (d)) coefficients are compared to the coefficients in the SDE (equation (13) of the main text). The blue curve is the approximation found by using the coefficient estimation technique and the red curve is the actual coefficient in the SDE. Clearly the agreement is good in both cases. In each case we take $N = 20$. For the coefficient estimation approach, in both cases, we take $\delta t = 1$ for estimating the drift coefficient and $\delta t = 0.1$ for estimating the diffusion coefficient. For the SDE we ran the simulations until each alignment value (of the $N + 1 = 21$ grid points) had been reached at least 100,000 times. For the individual-based model we ran the simulation for a total of 10,000,000 time units. In both scenarios we take reaction rates, $r_1 = 0.0225$, $r_2 = 0.0453$, $r_3 = 0.1664$, which correspond to the rates derived from fitting our analytical expressions for drift and diffusion to the averaged data.

[4] C. A. Yates, R. Erban, C. Escudero, I. D. Couzin, J. Buhl, I. G. Kevrekidis, P. K. Maini, and D. J. T. Sumpter, Proc. Natl. Acad. Sci. USA **106**, 5464 (2009).

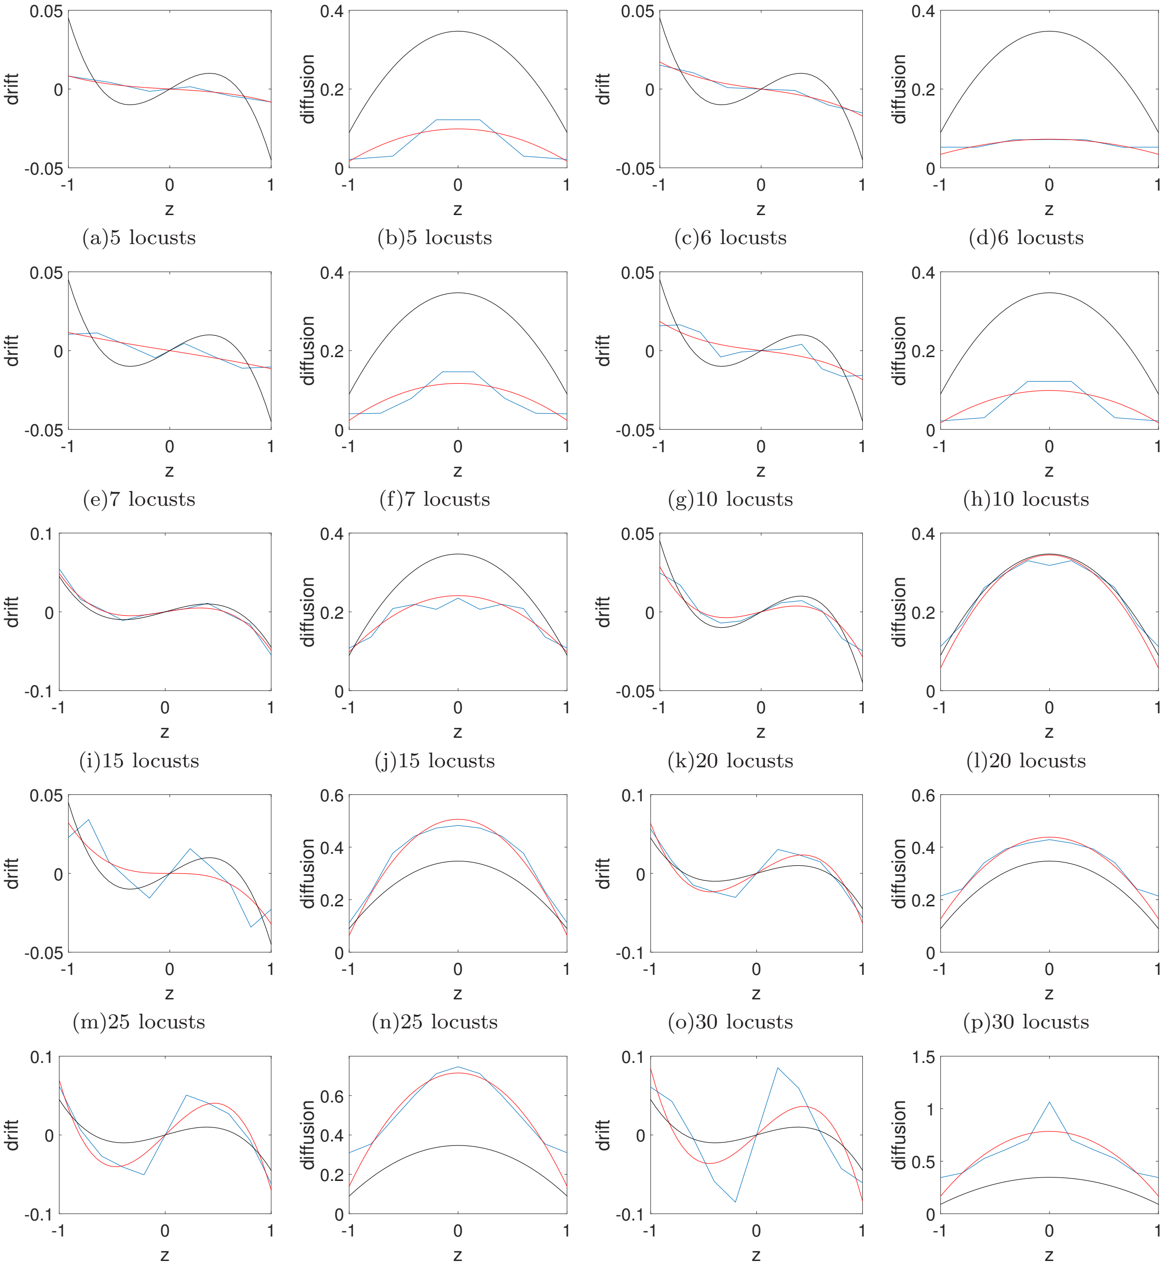


(a)5 locusts (b)5 locusts (c)6 locusts (d)6 locusts

(e)7 locusts (f)7 locusts (g)10 locusts (h)10 locusts

(i)15 locusts (j)15 locusts (k)20 locusts (l)20 locusts

(m)25 locusts (n)25 locusts (o)30 locusts (p)30 locusts

(q)35 locusts (r)35 locusts (s)40 locusts (t)40 locusts

FIG. S2. The drift coefficients and the diffusion coefficients (respectively) assumed to underlie the experimental data for a range of different locust numbers: (a) and (b) 5 locusts, (c) and (d) 6 locusts, (e) and (f) 7 locusts, (g) and (h) 10 locusts, (i) and (j) 15 locusts, (k) and (l) 20 locusts, (m) and (n) 25 locusts, (o) and (p) 30 locusts, (q) and (r) 35 locusts, (s) and (t) 40 locusts. The first figure of each pair represents the approximation of the drift coefficient and the second represents the approximation of the diffusion coefficient. The $x$-axis of each plot is the alignment, $z$. When calculating the drift coefficient the time interval, $\delta t$, was 4 frames (0.8 seconds), whereas for the diffusion coefficient we used a single frame (0.2 seconds).

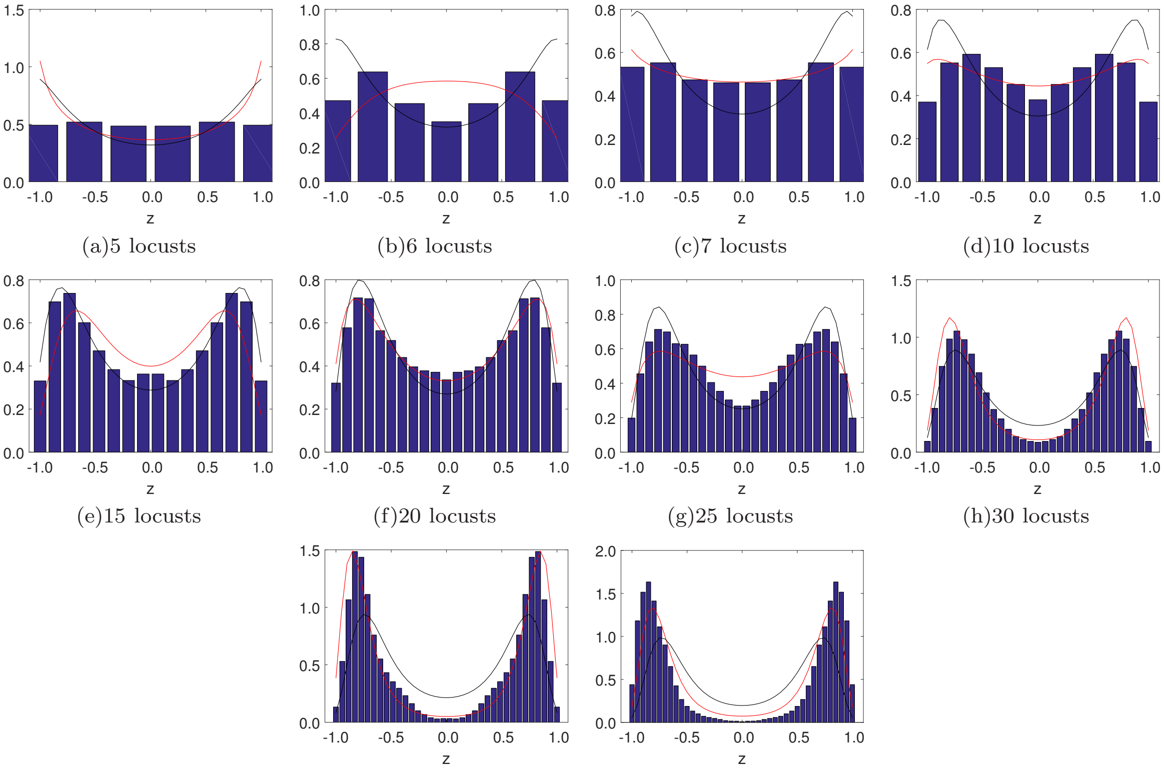

(a)5 locusts (b)6 locusts (c)7 locusts (d)10 locusts (e)15 locusts (f)20 locusts (g)25 locusts (h)30 locusts (i)35 locusts (j)40 locusts

FIG. S3. Experimentally observed stationary probability distributions (blue bars) compared to analytically predicted distributions with fitted parameters (red lines) and averaged fitted parameters (black lines) for different numbers of locusts. See Table I and Fig. 1 of the main text for reaction rates.
